# Supplementary material for: Derivation of a Local Volume-Averaged Model and a Stable Numerical Algorithm for Multi-Dimensional Simulations of Conversion Batteries
Source: arXiv:1909.07305 ancillary file (2019-09-16)
Supplement: Supplementary file 1 [file supplementary_material.pdf]

# Supplementary Materials for: Derivation of a Local Volume-Averaged Model and a Stable Numerical Algorithm for Multi-Dimensional Simulations of Zinc-Air Batteries

Tobias Schmitt<sup>a,b,c</sup>, Arnulf Latz<sup>a,b,c</sup>, Birger Horstmann<sup>a,b,c,\*</sup>

<sup>a</sup>German Aerospace Center, Pfaffenwaldring 38-40, 70569 Stuttgart, Germany

<sup>b</sup>Helmholtz Institute Ulm, Helmholtzstraße 11, 89069 Ulm, Germany

<sup>c</sup>Ulm University, Institute of Electrochemistry, Albert-Einstein-Allee 47, 89069 Ulm, Germany

## Contents

|                                                              |          |
|--------------------------------------------------------------|----------|
| <b>S1 Evolution Equations of Zinc-Air Battery Model</b>      | <b>1</b> |
| <b>S2 Domain Discretization</b>                              | <b>2</b> |
| <b>S3 Numerical Algorithms Tested</b>                        | <b>3</b> |
| <b>S4 Numerical Solvers for Linear and Nonlinear Systems</b> | <b>3</b> |

## S1. Evolution Equations of Zinc-Air Battery Model

In this paper, we analyze a zinc-air battery system, which we introduce in Ref. [1]. The governing equations for the volume fractions are [1]

$$\partial_t \varepsilon_{\text{Zn}} = -\nabla \cdot (\varepsilon_{\text{Zn}} \langle \dot{\mathbf{x}}_s \rangle) + V_{\text{Zn}}^{\text{mol}} \dot{\mathcal{P}}_{\text{Zn}}, \quad (\text{S1})$$

$$\partial_t \varepsilon_{\text{ZnO}} = -\nabla \cdot (\varepsilon_{\text{ZnO}} \langle \dot{\mathbf{x}}_s \rangle) + V_{\text{ZnO}}^{\text{mol}} \dot{\mathcal{P}}_{\text{ZnO}}, \quad (\text{S2})$$

$$\partial_t \varepsilon_l = -\nabla \cdot \langle \dot{\mathbf{x}}_l \rangle - \sum_{\beta_l} \bar{v}_{\beta_l} \nabla \cdot \langle N_{\beta_l} \rangle + \sum_{\beta_l} \bar{v}_{\beta_l} \dot{\mathcal{P}}_{\beta_l}, \quad (\text{S3})$$

with the molar volumes  $V_{\beta_s}^{\text{mol}}$ , partial molar volumes  $\bar{v}_{\beta_l}$ , the convection velocities  $\langle \dot{\mathbf{x}}_s \rangle$  and  $\langle \dot{\mathbf{x}}_l \rangle$  of the solid and liquid phase, non-convective flux terms  $N_{\beta_l}$ , and surface source terms  $\dot{\mathcal{P}}$ . The index  $\beta_l$  runs over all species. The convection velocities are calculated by Darcy's law for the fluid [2, 3] and a pseudo Darcy law for the solid

$$\langle \dot{\mathbf{x}}_s \rangle = \omega \nabla \bar{p}_s, \quad (\text{S4})$$

$$\langle \dot{\mathbf{x}}_l \rangle = \varepsilon_l \bar{\mathbf{x}}_l = -\frac{\varepsilon_l^2}{1 - \varepsilon_s} \frac{B_1^{\text{in}}}{\eta_l} \nabla \bar{p}_l, \quad (\text{S5})$$

with the pseudo-permeability  $\omega$ , the permeability  $B_1^{\text{in}}$ , the viscosity  $\eta_l$ , and the liquid pressure  $\bar{p}_l$ . The pressures  $\bar{p}_s$  and  $\bar{p}_l$  are expressed by the Leverett functions

$$\bar{p}_s = J_s(\varepsilon_s, \varepsilon_l, \varepsilon_g), \quad (\text{S6})$$

$$\bar{p}_{\text{atm}} - \bar{p}_l = J_l(\varepsilon_s, \varepsilon_l, \varepsilon_g). \quad (\text{S7})$$

\*Corresponding author

URL: birger.horstmann@dlr.de (Birger Horstmann)

with the atmospheric pressure  $\bar{p}_{\text{atm}}$ .

In our model assumption, the anode is made up of spherical zinc particles, with a porous zinc oxide shell around them. We denote them as primitive particles. Their number density  $\langle N_{\text{pp}} \rangle$  is determined by

$$\partial_t \langle N_{\text{pp}} \rangle = -\nabla \cdot (N_{\text{pp}} \bar{\mathbf{x}}_s). \quad (\text{S8})$$

The electrolyte is an aqueous potassium hydroxide solution, which consists of water, potassium, hydroxide, zincate, carbonate, and dissolved oxygen. The concentrations of the first two species are calculated by the constraints of electroneutrality and incompressibility. The latter four are unknowns, which are determined by (see Section 2.2.2)

$$\partial_t \langle c_{\gamma_1^-} \rangle = \nabla \cdot \langle D_{\gamma_1^-} \nabla c_{\gamma_1^-} \rangle - \nabla \cdot \left( \frac{t_{\gamma_1^-}}{z_{\gamma_1^-} F} \mathbf{j}_1 \right) + \nabla \cdot \left( \bar{c}_{\gamma_1^-} \frac{\varepsilon_1^2}{1 - \varepsilon_s} \frac{B_1^{\text{in}}}{\bar{\eta}_1} \nabla \bar{p}_1 \right) + \dot{\mathcal{P}}_{\gamma_1^-}. \quad (\text{S9})$$

$$\partial_t \langle c_{\gamma_1^0} \rangle = \nabla \cdot \langle D_{\gamma_1^0} \nabla c_{\gamma_1^0} \rangle + \nabla \cdot \left( \bar{c}_{\gamma_1^0} \frac{\varepsilon_1^2}{1 - \varepsilon_s} \frac{B_1^{\text{in}}}{\bar{\eta}_1} \nabla \bar{p}_1 \right) + \dot{\mathcal{P}}_{\gamma_1^0}. \quad (\text{S10})$$

$$\frac{2.73 j_1 |A_{\text{I,Zn}}|}{|A_{\text{ZnO}}^{\text{i}}|} = (1 - \varepsilon_f)^{3.5} \bar{D}_{\text{OH}^-} \frac{\bar{c}_{\text{OH}^-} - c_{\text{s,OH}^-}}{r_{\text{ZnO}}^0 - r_{\text{ZnO}}^{\text{i}}} \frac{r_{\text{ZnO}}^0}{r_{\text{ZnO}}^{\text{i}}}, \quad (\text{S11})$$

with the diffusion coefficients  $D_{\gamma_1^-}$ , transference numbers  $t_{\gamma_1^-}$ , charge numbers  $z_{\gamma_1^-}$ , and the electric current  $\mathbf{j}_1$ . The index  $\gamma_1$  runs over the primary species, which are hydroxide, zincate, carbonate, and oxygen in this case. The superscript differentiates between neutral, positive, and negative charges. Additionally, we model the surface concentration of hydroxide  $c_{\text{s,OH}^-}$ . Therefore, we use the surface areas of zinc  $|A_{\text{I,Zn}}|$  and zinc oxide  $|A_{\text{ZnO}}^{\text{i}}|$ , the inner and outer radii  $r_{\text{ZnO}}^{\text{i}}$  and  $r_{\text{ZnO}}^0$  of the zinc oxide shell, and the anodic reaction rate  $j_1$ . The surface areas and the radii are determined by a core-shell model, which describes the morphology of the anode [1]. The electric potentials  $\phi_1$  and  $\phi_s$  follow from

$$0 = \nabla \cdot \langle \kappa_1 \nabla \phi_1 \rangle + \nabla \cdot \left( \frac{\kappa_1}{F} \sum_{\gamma_1} \frac{t_{\gamma_1^-}}{z_{\gamma_1^-}} \left( \frac{\partial \mu_{\gamma_1^-}}{\partial c_{\gamma_1^-}} \right) \nabla c_{\gamma_1^-} \right) + \dot{\mathcal{P}}_{\text{q}}^{\text{l}}, \quad (\text{S12})$$

$$0 = \nabla \cdot \langle \kappa_s \nabla \phi_s \rangle + \dot{\mathcal{P}}_{\text{q}}^{\text{s}}. \quad (\text{S13})$$

with the conductivities  $\kappa_\alpha$  and the thermodynamic coefficients  $\partial \mu_{\gamma_1^-} / \partial c_{\gamma_1^-}$ .

A definition of the parameters is found in Ref. [1].

## S2. Domain Discretization

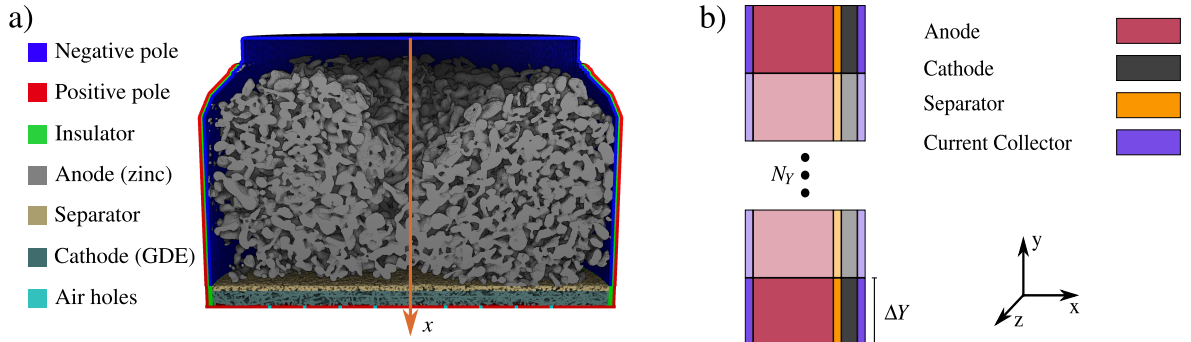

Figure S1: (a) Tomographic image of a zinc-air cell. (b) Domain discretization of the numerical stability simulations. We use one discretization unit for each domain in x-direction, resulting in a total of  $N_X = 5$  with a total extent of 5 mm. The number and size of the voxels in y-direction is varied in the numerical stability analysis. The geometry is symmetric in z-direction with  $N_Z = 3$  and an extent of 1 cm.

The domain discretization of the simulated zinc-air battery is shown in Fig. S1. We use a rectilinear grid and a rectangular geometry of the simulated battery. We define the through direction (connecting anode and cathode) as the

x-axis. It has a fixed thickness of 5 mm and is discretized with one voxel for each of the five domains. The z-direction is fixed to three equal-sized discretization units with a total extent of 1 cm. For our numerical stability analysis we vary the number of voxels  $N_Y$  and their size  $\Delta Y$ .

Table (S1) shows which variables are solved in which domain.

|                                                                                      | Anode | Cathode | Separator | Current collector |
|--------------------------------------------------------------------------------------|-------|---------|-----------|-------------------|
| $\varepsilon_{Zn}, \varepsilon_{ZnO}, c_{s,OH^-}, \bar{p}_s, \langle N_{pp} \rangle$ | X     |         |           |                   |
| $\varepsilon_1, \bar{p}_1, \bar{\phi}_1$                                             | X     | X       | X         |                   |
| $\bar{c}_{OH^-}, \bar{c}_{Zn(OH)_4^{2-}}, \bar{c}_{CO_3^{2-}}, \bar{c}_{O_2^l}$      | X     | X       | X         |                   |
| $\bar{\phi}_s$                                                                       | X     | X       |           | X                 |

Table S1: Connection of the variables to the geometrical domains (see Fig. S1d).

### S3. Numerical Algorithms Tested

To improve the robustness of the solver, we test multiple algorithms. Among them are backward differentiation formula (BDF), Adams-Moulton (AM) methods, and explicit and implicit Runge-Kutta schemes for the time integration. For the solution of the linearized system of equations, we test GMRES, BiCGSTAB, PARDISO [4, 5, 6, 7], various preconditioners [8], and different multi-grid cycles. The best result is achieved with an ILU preconditioned BiCGSTAB, with a K-cycle as multi-grid strategy and a Crank-Nicolson scheme (first order Adams-Moulton) as time integration algorithm. A damped Jacobian nonlinear-iteration improves the stability slightly by damping the high frequency errors, but it increases the number of iterations and thus the computation time. Convective transport terms are implemented by a first order upwind scheme. Reducing the number of differential algebraic equations by using the partial time derivative of the pressure equation ( $\partial_t \bar{p}_1 = (\partial_{\varepsilon_1} J_1)(\partial_t \varepsilon_1) + (\partial_{\varepsilon_1} J_1)(\partial_t \varepsilon_1)$ ) has no effect. Thus, we stick to Eq. (S7), which is easier to handle. Using an operator-splitting technique [8, 9, 10], by solving first the diffusion-reaction problem and then adding the convective transport reduces  $\Delta t_{\max}$ . Commonly used algorithms in computational fluid dynamics with convective transport are the SIMPLE and SIMPLER method to handle the pressure-velocity coupling [11, 12]. Due to the different structure of equations, they cannot be applied here. In numerical simulations of general relativistic problems it is necessary to split a variable into two [13]. This reduces the coupling between the variables and makes the Jacobi matrix sparser. Analogous to that we define the velocity  $\bar{x}_1$  on the cell walls (staggered grid) and define  $\partial_t \varepsilon_1$  as an independent variable. However, this approach shows no improvement. The same holds for a change of the unknowns (from  $\{\varepsilon_1, \bar{c}_{\gamma_1}\}$  to  $\{\varepsilon_1, \langle c_{\gamma_1} \rangle\}$ ) and thus solving the equation  $\varepsilon_1 = \sum_{\beta_1} \bar{\nu}_{\beta_1} \langle c_{\beta_1} \rangle$  instead of Eq. (55).

Inspired by operator-splitting techniques and the SIMPLE method, we develop a new algorithm, which is based on a decoupled SOE. We solve the subsystems sequentially after each other until the solution converges. We call this method a Sequential Semi-Implicit (SSI) Algorithm (see Section 3.3). This method is the only known algorithm, which increases the stability by orders of magnitude (in measures of  $\Delta t_{\max}$ ).

### S4. Numerical Solvers for Linear and Nonlinear Systems

We split all equations in a part containing the time derivative (LHS) and a part containing all flux and source terms (RHS). The right hand side of all equations are discretized by a first order Adams-Moulton method (Crank-Nicolson). This method is second order accurate in  $\Delta t$  [10, 7]. Convective terms are incorporated by a first order upwind scheme. We call this the linearized system. It is solved by a multi-grid (K-cycle) BiCGSTAB algorithm. As preconditioner, we use an incomplete LU decomposition. The solver on the coarsest level is PARDISO.

Since we solve an implicit system of equations, we have to update the unknowns after each successful call of the linear solver and repeat this process. This is called the nonlinear system and is solved by an Newton method with a dynamic Jacobian damping. After each update of the nonlinear system, we check if all variables are within a physical

and predefined range. In the case of overshoots of the solution, we reduce the damping factor. The nonlinear iteration is repeated until the solution converges against a solution and we perform another time step.

## References

- [1] T. Schmitt, T. Arlt, I. Manke, A. Latz, B. Horstmann, Zinc electrode shape-change in secondary air batteries: A 2D modeling approach, *Journal of Power Sources* 432 (2019) 119–132. doi:10.1016/j.jpowsour.2019.126649.
- [2] B. Horstmann, T. Danner, W. G. Bessler, Precipitation in aqueous lithium-oxygen batteries: a model-based analysis, *Energy & Environmental Science* 6 (4) (2013) 1299–1314. doi:10.1039/c3ee24299d.
- [3] S. Whitaker, Flow in porous media I: A theoretical derivation of Darcy’s law, *Transport in Porous Media* 1 (1) (1986) 3–25. doi:10.1007/BF01036523.
- [4] O. Schenk, K. Gärtner, Solving unsymmetric sparse systems of linear equations with PARDISO, *Future Generation Computer Systems* 20 (3) (2004) 475–487. doi:10.1016/j.future.2003.07.011.
- [5] PARDISO 6.0 Solver Project, <https://www.pardiso-project.org/>. Last visited 2019-01-08.
- [6] R. J. LeVeque, *Finite Difference Methods for Ordinary and Partial Differential Equations*, Society for Industrial and Applied Mathematics, 2007. doi:10.1137/1.9780898717839.
- [7] A. Quarteroni, R. Sacco, F. S. Springer, *Numerical Mathematics*, 2nd Edition, Springer-Verlag, 2000. doi:10.1007/b98885.
- [8] Y. Saad, *Iterative Methods for Sparse Linear Systems*, [https://www-users.cs.umn.edu/~saad/IterMethBook\\_2ndEd.pdf](https://www-users.cs.umn.edu/~saad/IterMethBook_2ndEd.pdf). Last visited 2019-01-08.
- [9] A. Quarteroni, A. Valli, *Numerical approximation of partial differential equations*, 1st Edition, Springer-Verlag, 1994. doi:10.1007/978-3-540-85268-1.
- [10] A. Quarteroni, *Numerical Models for Differential Problems*, 2nd Edition, Springer-Verlag, 2012. doi:10.1007/978-88-470-5522-3.
- [11] S. V. Patankar, *Numerical heat transfer and fluid flow*, Hemisphere Publishing Corporation, 1980. doi:10.1002/cite.330530323.
- [12] J. H. Ferziger, M. Perić, *Computational Methods for Fluid Dynamics*, 1st Edition, Springer-Verlag, 2002. doi:10.1007/978-3-642-56026-2.
- [13] T. W. Baumgarte, S. L. Shapiro, *Numerical relativity: solving Einstein’s equations on the computer*, Cambridge University Press, 2010. doi:10.1017/CB09781139193344.
